# Supplementary material for: PointAR: Efficient Lighting Estimation for Mobile Augmented Reality
Source: arXiv:2004.00006 source file (2020-07-17)
Supplement: Supplementary file 1 [file appendix.tex]

\section{Spatially Variant Lighting Estimation}
\label{sec:appendix}

Figure~\ref{fig:spatial_variant} shows the rendering examples by leveraging \sysname to estimate lighting at locations with spatially variant lighting conditions. For each image, aside from the ground truth location, we additionally chose two more rendering locations that exhibited visually different lighting conditions. For each image in the first row, three Stanford bunnies were lit by the \shc estimated by \sysname. We observe visually satisfying rendering effects for 3D objects at different locations. 

%%%
\begin{figure}[t]
\centering
\includegraphics[width=0.95\textwidth]{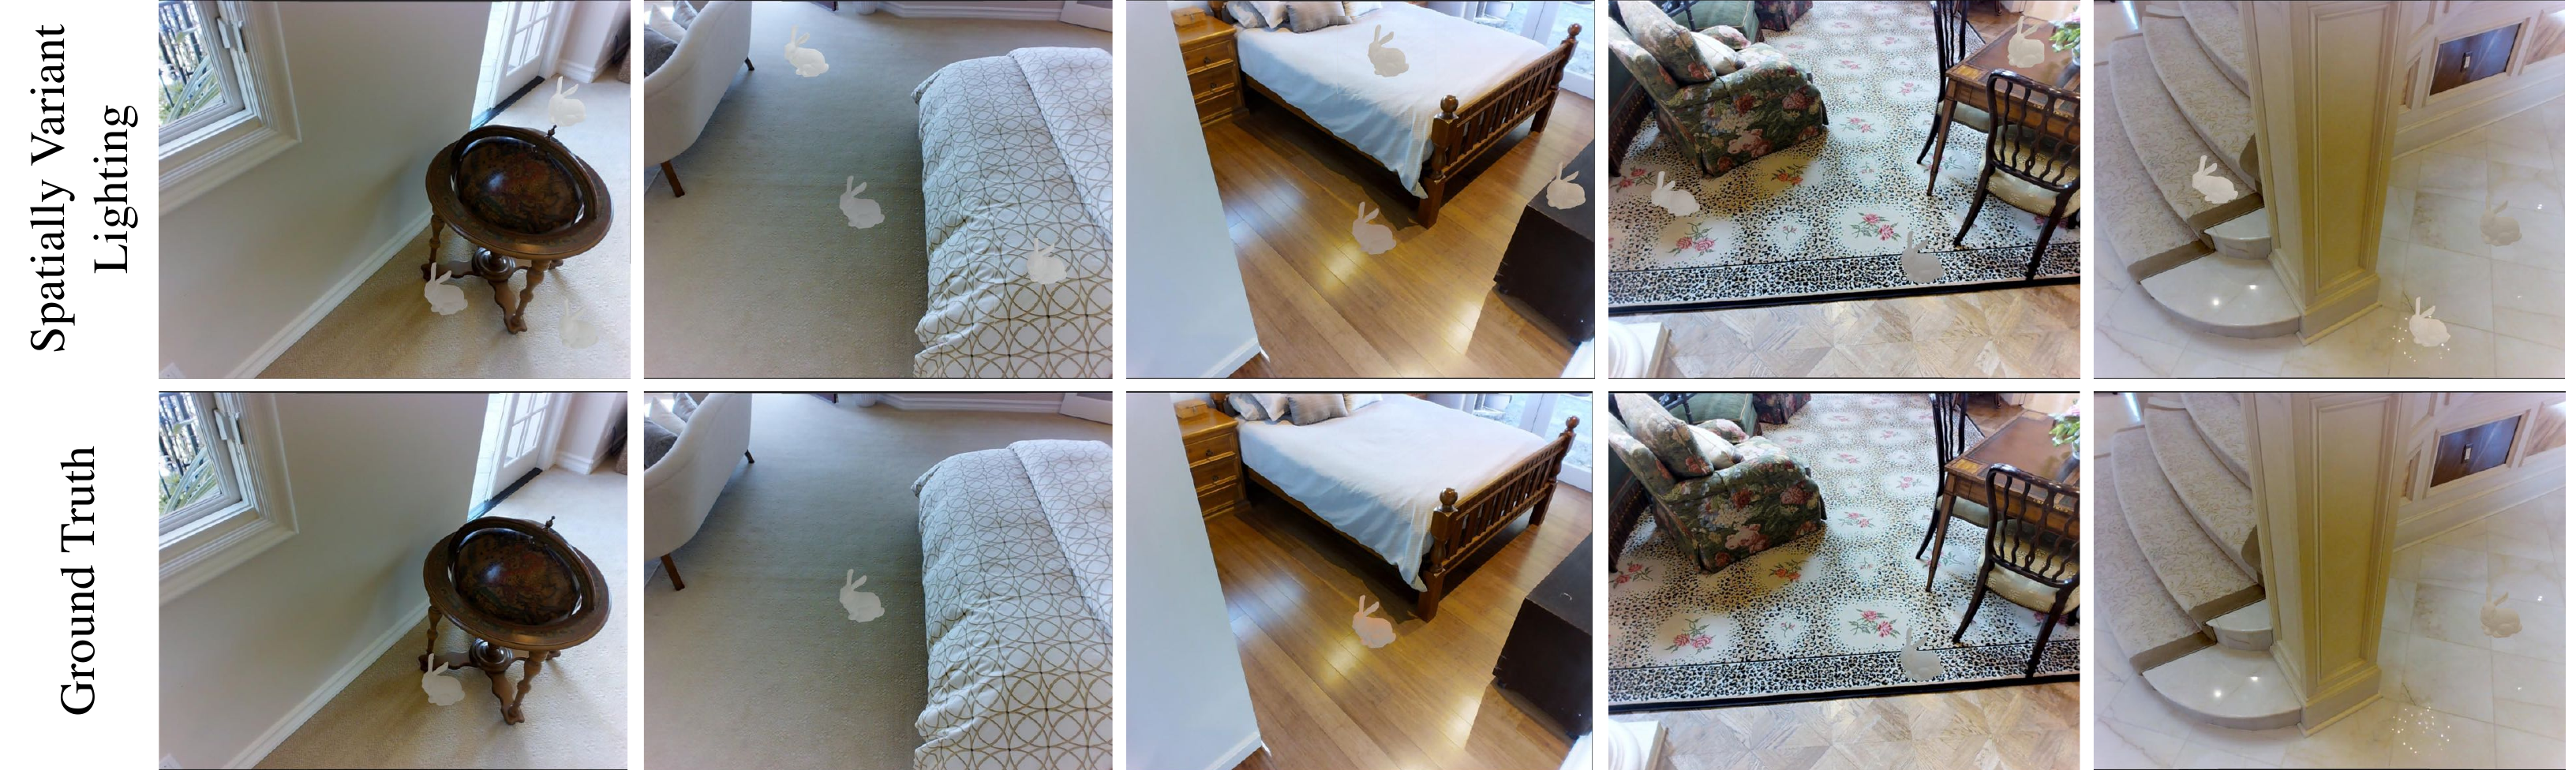}
\caption{\textbf{Rendering examples of \sysname in spatially variant lighting conditions}.
Row 1 shows the Stanford bunnies that were lit using the \shc predicted by \sysname. 
Row 2 shows the ground truth rendering results.
}
\label{fig:spatial_variant}
\end{figure}
%%%
